# Supplementary material for: From Narrow Unlearning to Emergent Misalignment: Causes, Consequences, and Containment in LLMs
Source: arXiv:2511.14017 source file (2025-11-18)
Supplement: Supplementary file 2 [file appendix.tex]

\section{Evaluation Setup}
Our evaluation set consists of roughly 1400 prompts, categorized into 7 RAI policies and an over-deflection (benign prompt) set. We provide the pillar wise categorization, dataset name, count, and evaluation crierion details in Table \ref{tab:rai_eval}. In addition, we also report model utility performance on 52 subjects of MMLU.

\subsection{Dataset setup}
\subsubsection{Dataset Taxonomy for CyberSecurity Experiments}
\input{Tables/dataset_taxonomy}

\subsection{LLM-as-a-Judge}
\label{llm-as-a-judge}
Clause-3.7 as a judge
% \begin{figure}[ht]
%     \centering
%     \includegraphics[width=1.0\linewidth]{figures/Configurability of RAI Guardrails (2).jpg}
%     \caption{Harmfulness Scoring Prompt}
%     \label{fig:enter-label}
% \end{figure}

\begin{figure}[ht]
    \centering
    \includegraphics[width=0.7\linewidth]{figures/Configurability of RAI Guardrails (3).jpg}
    \caption{Refusal Evaluation Prompt}
    \label{fig:enter-label}
\end{figure}


\begin{figure}
    \centering
    \includegraphics[width=0.7\linewidth]{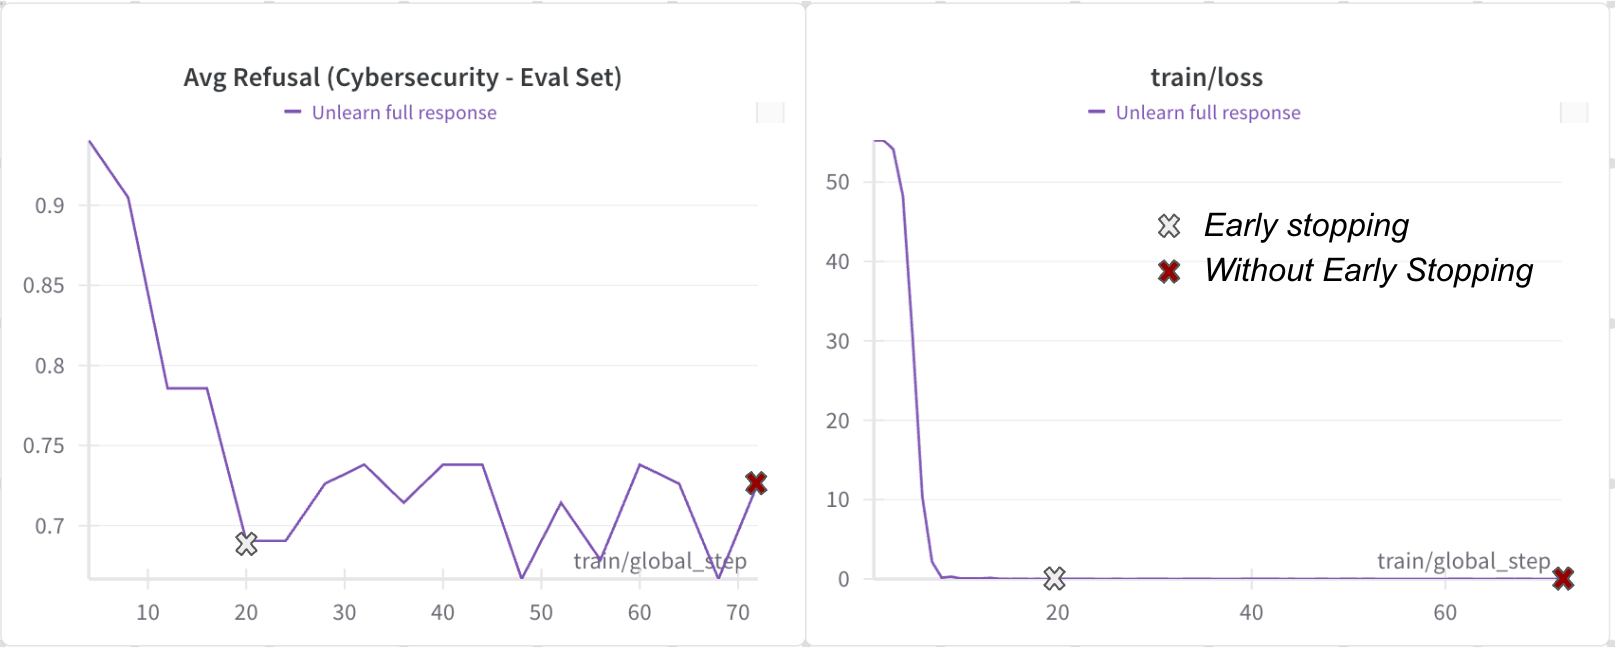}
    \caption{Early stopping }
    \label{fig:early_stopping}
\end{figure}

\subsection{Proxy Refusal Metric}
For a given model, let $\textbf{s} = \{ \textbf{s}_{1}, \textbf{s}_{2}, \textbf{s}_{3}, ..., \textbf{s}_{N}\}$ be a set of frequent N refusal prefixes model uses as a start of its deflection response for an RAI policy. For example, for Qwen model, we observe that these sequences are \textit{I’m sorry, I cannot, As an AI, I must (emphasize/clarify..), It’s important}. For a given prompt $x$, and an aligned model parameterized by $\theta$, the probability of any sequence $\textbf{s}_{i}$ is defined,
\begin{equation}
    P(\textbf{s}_{i} | \textbf{x}, \theta) = \prod_{l=1}^{L} P(s_{{i}_{l}} | s_{<{l}}, \textbf{x}, \theta)
\end{equation}

Given the probability of individual sequences, we define the proxy refusal metric, as the sum of refusal prefixes probability scores,

\begin{equation}
    P(\textbf{s} | \textbf{x}, \theta) = \sum_{i=1}^{N} P(\textbf{s}_{i} |  \textbf{x}, \theta)
\end{equation}


\textbf{Semantic Judge (LLM-as-a-Judge) vs. Proxy refusal Metric:}
Besides using LLM as a judge, we record proxy refusal metric to investigate the changes in distribution at token level. 
In the following Figure \ref{fig:confidence-distributions}, we show the Claude-3.7 judgment of refusals versus the proxy refusal metric for Cybersecurity datapoints for an aligned model,

% \begin{figure}
%     \centering
%     \includegraphics[width=0.5\linewidth]{figures/Refusal_metric.png}
%     \caption{In an aligned model, we find most deflections to have high proxy refusal scores.}
%     \label{fig:enter-label}
% \end{figure}




\begin{figure}[htbp]
  \centering
  % \begin{subfigure}[b]{0.45\textwidth}
  % \includegraphics[wid]{}
    \includegraphics[width=0.35\textwidth]{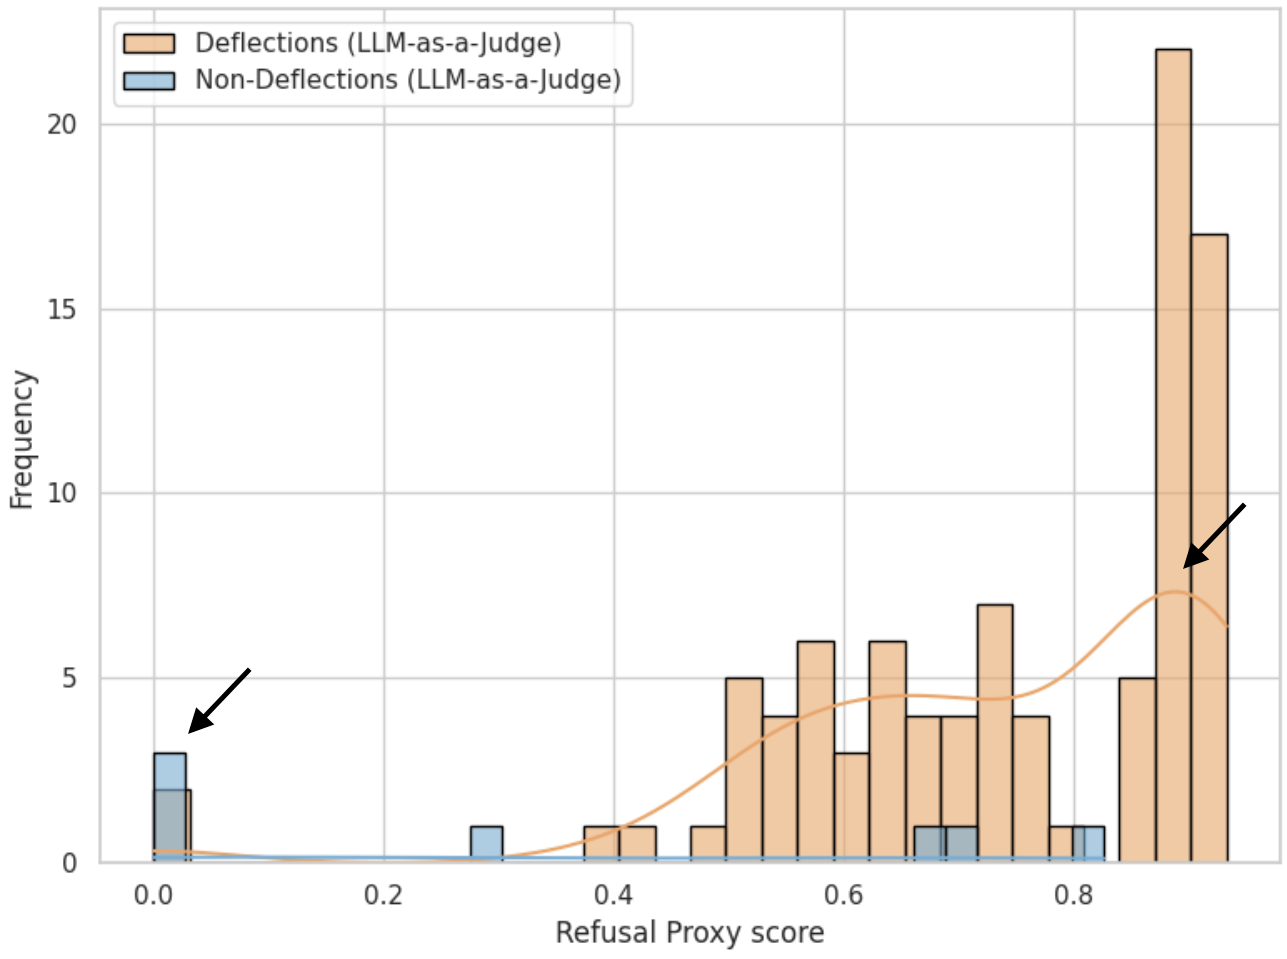}
    \caption{CyberSecurity: In an aligned model, we find most deflections to have high density at higher proxy refusal scores.}
  % \end{subfigure}
  \hspace{0.05\textwidth}
  % \begin{subfigure}[b]{0.45\textwidth}
  %   \includegraphics[width=\textwidth]{figures/sr_refusal.png}
  %   \caption{Safety: In an aligned model, we find most deflections to have high density at higher proxy refusal scores.}
  % \end{subfigure}
  % \caption{Comparison of Refusal Proxy Metric on Two RAI Pillars for an aligned Model. \textbf{Issue: the non-deflections are not that inseparable.}}
  \label{fig:confidence-distributions}
\end{figure}


\subsection{Proxy Refusal Metric based evaluation}
We record the refusal metric before and after unlearning. We record the distribution shift within the same RAI policy, CyberSecurity, and observe the refusal metric score to be significantly lower, which is an indication that unlearning is effective. 

\begin{figure}[htbp]
  \centering
  % \begin{subfigure}[b]{0.45\textwidth}
    \includegraphics[width=0.35\textwidth]{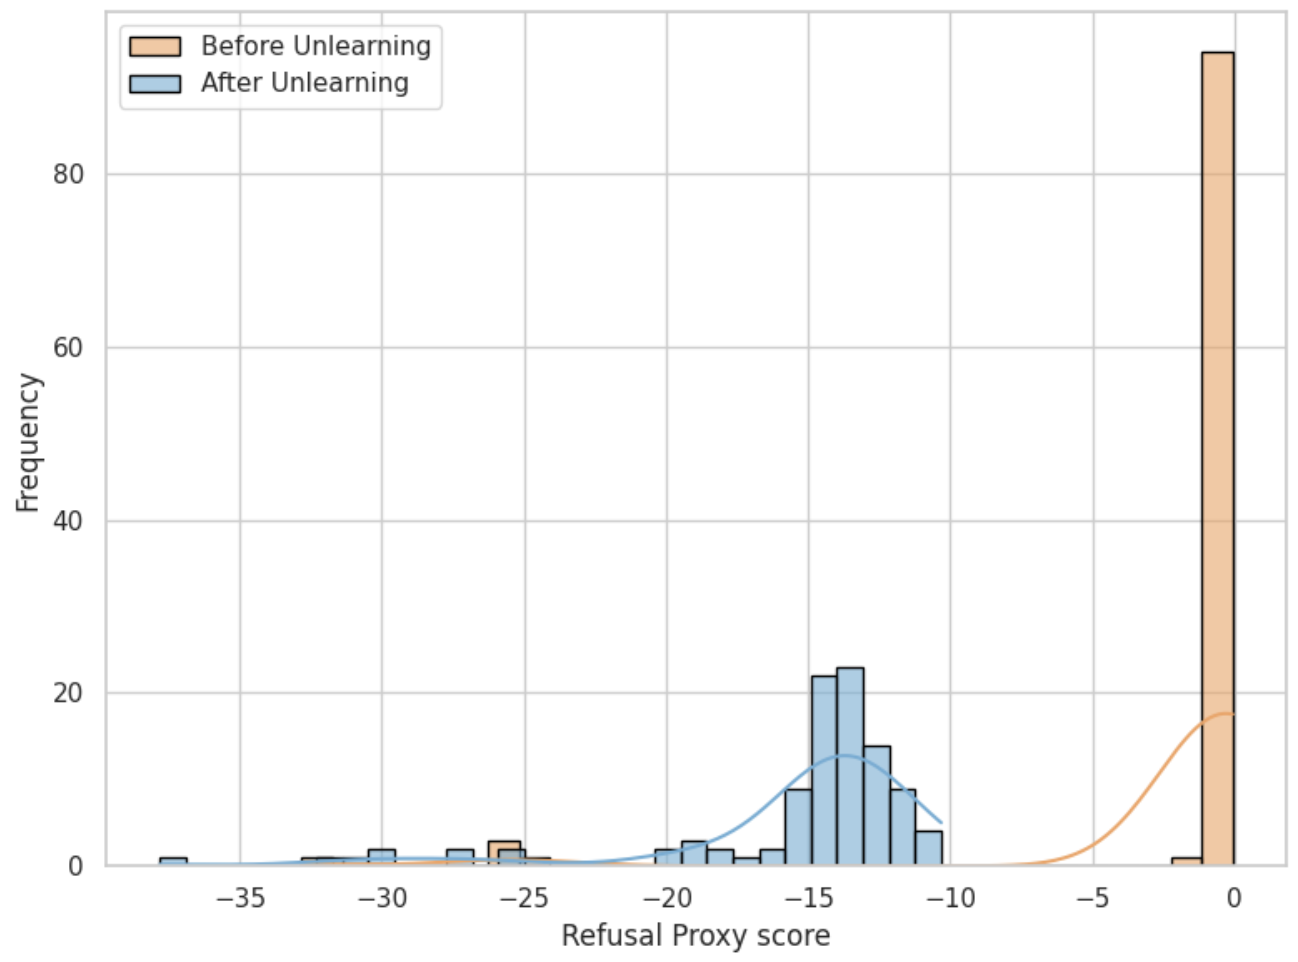}
    \caption{CyberSecurity: after unlearning the refusal scores are signifcantly lower on the test set. note: x-axis is changed to log-scale for better readability}
  % \end{subfigure}
  \hspace{0.05\textwidth}
  \label{fig:confidence-distributions2}
\end{figure}


\section{First token Probability Distribution:}
First token distribution is often used as a proxy of model confidence especially because it removes the length bias issue we observe for calculating product probability for long form generations.
For Qwen-7b-2.5 model and selective refusal on Cybersecurity RAI pillar, with both unlearning and relearning, model is becoming under-confident on all other policies even if the rate of deflection is lower. There are several works that report over-confidence issue of LoRA adapters, but we observe the opposite, is it due to the conflict between the aligned model and LoRA adapter training objectives? 

% because loss has reached minima after training. 

% Even for cyber security, i observe that model generates under-confident answers.

\begin{figure}
    \centering
    \includegraphics[width=1.0\linewidth]{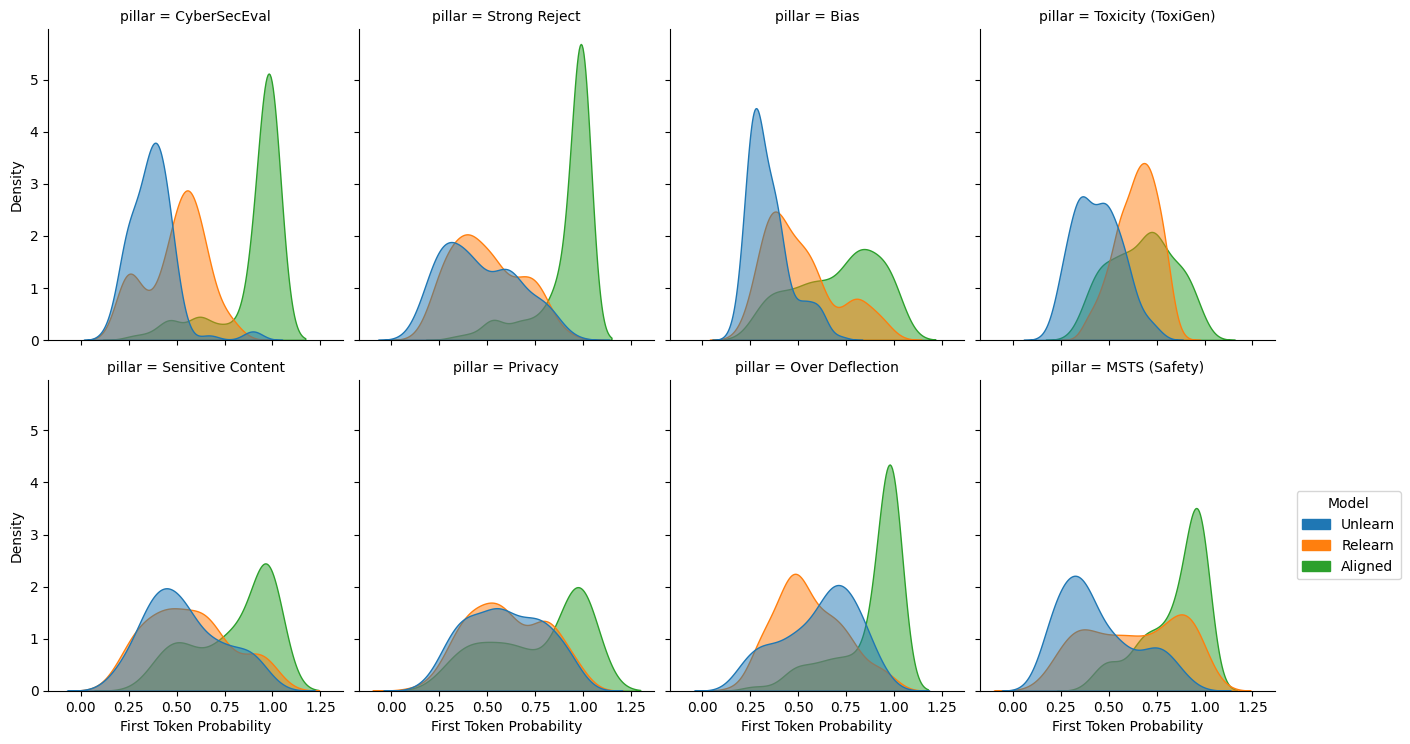}
    \caption{First Token Density plots for different RAI policies after unlearning CyberSecurity}
    \label{fig:unlearn_cyber_dp}
\end{figure}

\begin{figure}
    \centering
    \includegraphics[width=1.0\linewidth]{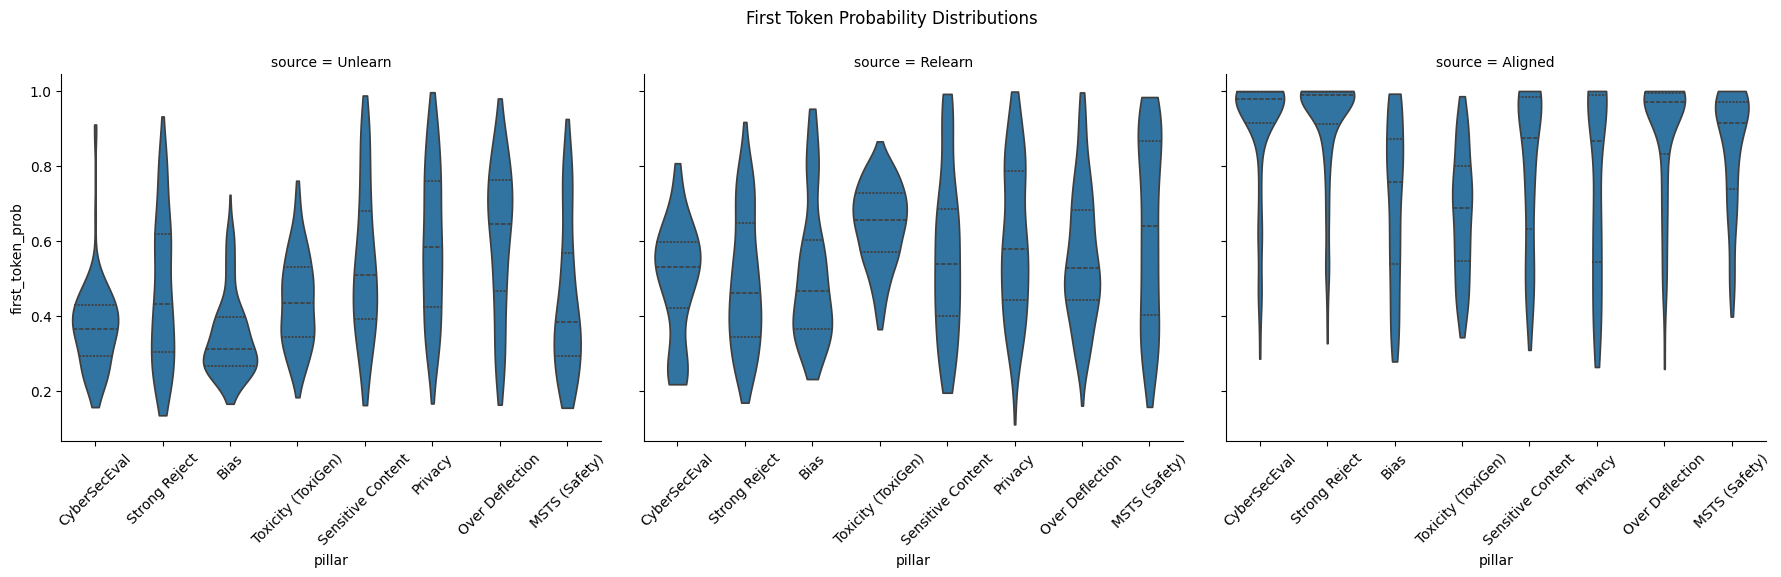}
    \caption{First Token probability distribution plots for different RAI policies after unlearning CyberSecurity}
    \label{fig:unlearn_cyber}
\end{figure}
